# Supplementary material for: Interplay of rearrangements, strain, and local structure during avalanche propagation
Source: arXiv:2009.11414 source file (2020-09-23)
Supplement: Supplementary file 1 [file supplementary.pdf]

# Supplementary Information for Interplay of softness and rearrangements during avalanche propagation

Ge Zhang, Sean Ridout, and Andrea J. Liu*
Department of Physics and Astronomy,
University of Pennsylvania, *Philadelphia PA 19104*

* ajliu@physics.upenn.edu

## I. STEEPEST DESCENT WITH ON-THE-FLY ADJUSTMENT OF THE STEP SIZE

We follow the energy minimization process from the top to the bottom of an energy drop using steepest descent in order to accurately capture avalanche propagation in an over-damped system. However, steepest descent with a fixed step size is either extremely inefficient or inaccurate. We therefore adjust step sizes during minimization with the following protocol:

- Start with a step size of $s = 10^{-3}$ (in units of small particle diameter)
- Let the particle positions be $\mathbf{r}^N$, the total potential energy be $U(\mathbf{r}^N)$, and the potential energy change between two steps be $\delta U$ [S1]. If the difference between $\delta U$ and $s|U'(\mathbf{r}^N)|$ exceeds 10%, we abort this move (*i.e.,* do not change $\mathbf{r}^N$) and reduce $s$ by a factor of two.
- If the difference between $\delta U$ and $s|U'(\mathbf{r}^N)|$ is less than 5%, we increase $s$ by 10% to increase efficiency.

Overall, this energy minimization algorithm requires roughly four times more evaluations of $U(\mathbf{r}^N)$ and $U'(\mathbf{r}^N)$ to converge than the FIRE minimization algorithm.

## II. SAMPLING SNAPSHOTS DURING ENERGY MINIMIZATION

During energy minimization, we save intermediate configurations for further analysis. These intermediate configurations are spaced to be equi-distant in configuration space, with the distance between adjacent frames chosen to be $\sqrt{\sum_i^N \delta\mathbf{r}_i^2} = 0.15$. This choice is made so that movies generated from such frames are smooth (see supplementary movie).

For comparison we also saved intermediate configurations spaced according to a fixed decrease of energy or time elapsed. Here "time" is simply defined as $\sum s/|U'(\mathbf{r}^N)|$ since we use over-damped dynamics. However, these schemes resulted in uneven distribution of $D^2_{\mathrm{min}}$ along the trajectory. In other words, we find that the distributions of $D^2_{\mathrm{min}}$ for the first and second halves of an avalanche are the same for the first sampling scheme but not for the latter two. Since an even distribution of $D^2_{\mathrm{min}}$ is important in training the machine-learning

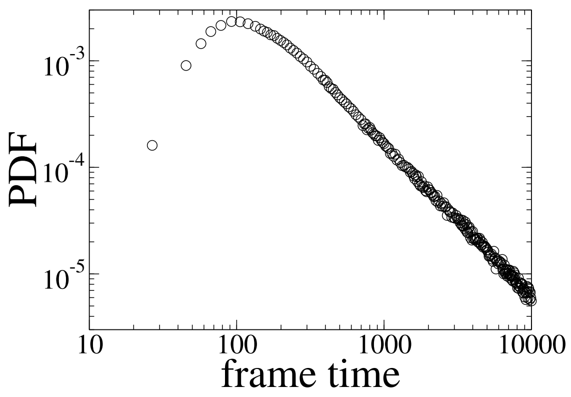


FIG. S1. The probability density function (PDF) of the time interval between two frames.

TABLE I. Parameters in defining training sets.

| $d_{\text{soft, small}}$ | $d_{\text{soft, large}}$ | $d_{\text{hard, small}}$ | $d_{\text{hard, large}}$ | $\delta\epsilon$ |
|---|---|---|---|---|
| 0.005 | 0.003 | 0.002 | 0.002 | 0.15 |
| 0.0025 | 0.0015 | 0.004 | 0.004 | 0.15 |

algorithm, we chose the first sampling scheme. The distribution of the time interval between frames in presented in Fig. S1.

## III. CALCULATING SOFTNESS

Following previous work [S2], we calculate softness using the support-vector machine (SVM) algorithm with a linear kernel. To select the training set, we identify 7500 rearranging particles with $D^2_{\text{min}} > d_{\text{soft}}$ between two adjacent frames during energy minimization and 7500 non-rearranging particles with $D^2_{\text{min}} < d_{\text{hard}}$ between two energy-minimized frames separated by a shearing strain of $\delta\epsilon$. We use two sets of parameters listed in Table I.

For a good training set we need non-rearranging particles that do not rearrange over a long period of time prior. To obtain such particles, we simulated smaller systems over a longer shear strain window. Specifically, we generated 20 trajectories with $N = 4000$, $\delta\epsilon = 10^{-4}$, and $\epsilon_{end} = 2$. After training, we verified that $P(S)$ and $P(S|R)$ are nearly the same and that $P_R(S)$ is very similar for the two system sizes (see Fig. S2).

After selecting training sets, we calculate structure functions. Although previous work employed two-body as well as three-body structure functions, we found the three-body ones computationally expensive and not very helpful (resulting in less than 1% increase

TABLE II. Structure function placements.

| $r_{\text{m, small}}$ | $r_{\text{m, large}}$ |
|---|---|
| $0.8, 0.8 \times 1.04, 0.8 \times 1.04^2, \cdots, 9.85$ | $1, 1.04, 1.04^2, \cdots, 9.72$ |
| $0.8, 0.8 \times 1.04, 0.8 \times 1.04^2, \cdots, 5.91$ | $1, 1.04, 1.04^2, \cdots, 5.84$ |
| $0.8, 0.8 \times 1.04, 0.8 \times 1.04^2, \cdots, 2.92$ | $1, 1.04, 1.04^2, \cdots, 3.00$ |
| $0.8, 0.9, 1.0, \cdots, 10.0$ | $1.0, 1.1, 1.2, \cdots, 10.0$ |
| $0.8, 0.9, 1.0, \cdots, 6.0$ | $1.0, 1.1, 1.2, \cdots, 6.0$ |
| $0.8, 0.9, 1.0, \cdots, 2.9$ | $1.0, 1.1, 1.2, \cdots, 2.9$ |

in the accuracy), and thus neglected them, consistent with Ref. [S2]. To further improve computational efficiency, we use linear radial structure functions:

$$G_m(i) = \sum_j g_{m,ij}, \tag{S1}$$

where

$$g_{m,ij} = \begin{cases} 1 - (r_{ij} - r_m)/(r_{m-1} - r_m), & \text{if } r_{m-1} < r < r_m, \\ 1 - (r_{ij} - r_m)/(r_{m+1} - r_m), & \text{if } r_m < r < r_{m+1}, \\ 0, & \text{otherwise,} \end{cases} \tag{S2}$$

and $r_m$ is the location of the $m$th radial function. The training and testing accuracy is the same for these structure functions as for the structure functions with Gaussian smoothing. We use multiple sets of $r_m$ listed in Table II.

Finally, we adopt the ensemble method to calculate softness. In machine learning, "ensemble" refers to training multiple hyperplanes (or neural networks, decision trees, etc.) and averaging their predictions. For each combination of training set (Table I) and structure function placement (Table II), we train 5 hyperplanes. This yields 60 hyperplanes (per species) in total. The validation accuracy for individual hyperplanes varies in a small range of $0.878 - 0.926$. The final softness of a particle is the average of the signed distance to all hyperplanes.

In the main text, a rearranger is defined using the smaller $D^2_{\text{min}}$ threshold, *i.e.*, $d_{\text{soft, small}} = 0.0025$ and $d_{\text{soft, large}} = 0.0015$. Finally, we note that when studying the strain and softness change caused by a rearrangement (Figs. 2 and 5 of the main text), we focus on frames that (1) contain only one rearranger; and (2) contain no particle that is

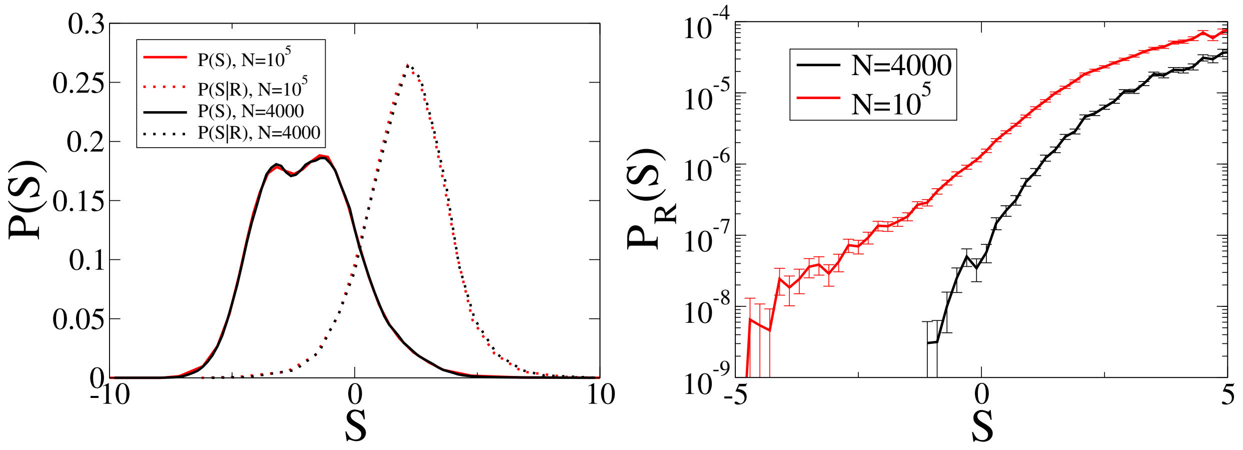


FIG. S2. Sanity checks for machine-learned softness. (left) The distribution of softness for all particles(solid curves) and for rearranging particles (dotted curve). The distinction between the two distributions is clear and shows that rearranging particles tend to have significantly higher softnesses. The results for the two different system sizes, $N = 4000$ and $N = 10^5$, are nearly indistinguishable. (right) The probability that a particle is rearranging, $P_R$, as a function of its softness. As $S$ increases, $P_R$ increases by several orders of magnitude for both system sizes, verifying the high correlation between softness and rearrangements. The reason for the system size dependence are twofold. First, our hyperplanes are fitted to data from the $N = 4000$ system but not the $N = 10^5$ system, and may suffer from overfitting, resulting in artificially steeper $P_R(S)$. Second, our time resolution is tuned so that the number of rearranging particles per frame, $N_R$, is no more than a few. Therefore $N_R$ does not scale linearly with the system size. This effect would contribute a constant difference in $P_R$ for different system sizes.

not close to the rearranger (distance greater than 5) that has $D^2_{\text{min}} > 0.01 d_{\text{soft}}$. The latter criterion is introduced to exclude frames with multiple rearrangements.

## IV. $P_R$ FOR A GIVEN SOFTNESS IS ARRHENIUS AT POSITIVE TEMPERATURE

Here we show that the softness values we obtained is strongly correlated with rearrangements not only at zero temperature, but also thermal unsheared systems above the glass transition. We perform molecular dynamics simulations of a 10,000-particle system with the same composition, density, and interactions as the quasistatically-sheared systems at

temperatures $k_BT = 2.6 \times 10^{-4}$, $3 \times 10^{-4}$, $3.5 \times 10^{-4}$, $4 \times 10^{-4}$, and $5 \times 10^{-4}$, using a time step $\delta t = 0.02$. Starting from square-lattice initial conditions, we first equilibrate the system at a much higher temperature ($k_BT = 10^{-3}$) for $10^7$ time steps, then equilibrate at the desired temperature for $5 \times 10^7$ time steps. We then save configurations every $10^3$ time steps and accumulate $10^4$ snapshots. We define rearrangers as those with $D^2_{\mathrm{min}} > 0.5$ between the inherent structures (local energy minima) of two adjacent snapshots, and calculate the rearranging probability, shown in Fig. S3. As we can see, for a given softness, the probability of rearranging follows the Arrhenius relation $P_R = A\exp(-E_a/k_BT)$, where $E_a$ is the activation energy. This observation, consistent with our earlier observations for Kob-Andersen systems [S2] and polycrystalline metals [S3], confirms that softness is related to the energy barrier for rearrangements in this system.

We have extracted $E_a$ as a function of softness by numerically fitting the above results. At the same time, we estimate $E_a$ from the athermal quasistatic simulations, as follows. Recall that we calculated the amount of shear strain $\tilde{\epsilon}$ needed to trigger a rearrangement (Fig. 6 of the main text). The elastic energy stored in the region that will rearrange is

$$E_a = \frac{1}{2} V G \tilde{\epsilon}^2, \tag{S3}$$

where $V$ is the volume of the deformed region and $G$ is the shear modulus. We numerically measured $G = 0.1155$ for our system, and choose $V = \pi$ (in units of small particle diameter) as a reasonable assumption. We compare the activation energies extracted from these two types of simulations in Fig. S4, and find that they are quantitatively similar as shown. The weaker softness dependence in thermal systems may arise because we are using a hyperplane trained at $T = 0$ to describe systems at $T > T_g$. It is remarkable that we still achieve a reasonable accuracy, but not surprising that the energy barrier dependence is smeared out. Indeed, Fig. S4 shows that when we train a hyperplane on $T > T_g$ rearrangements, we obtain a range of energy barriers that is much more similar (up to a factor of order unity) to what we estimate at $T = 0$.

## V. VERIFYING MAIN RESULTS IN THREE DIMENSIONS

To verify that our main results hold in three dimensions, we generated 10 trajectories with $N = 12000$, $\delta\epsilon = 10^{-4}$, and $\epsilon_{end} = 1$ for training; and 2 trajectories with $N = 10^5$,

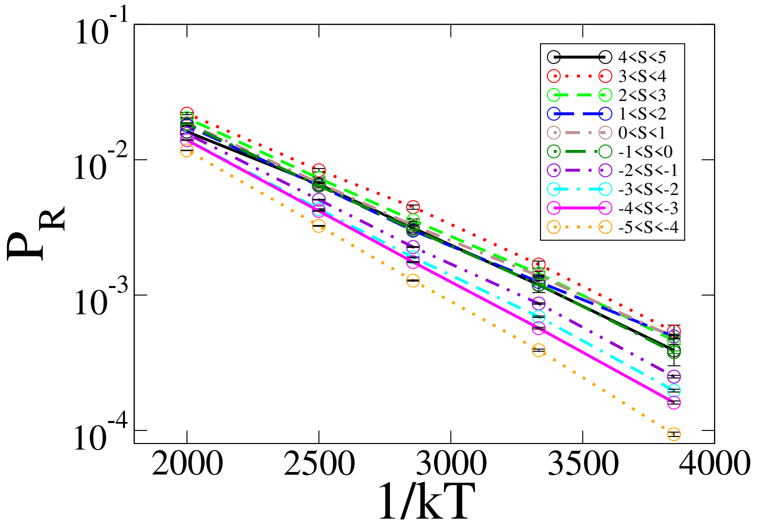


FIG. S3. The probability that a particle with a given softness is rearranging in a molecular-dynamics simulation, as a function of the inverse temperature.

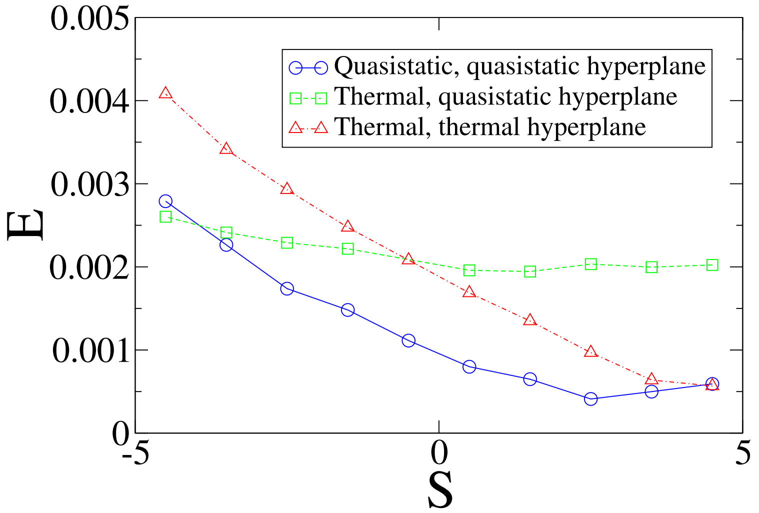


FIG. S4. Activation energy for rearrangements as a function of softness, (blue) extracted from quasistatic simulations using quasistatic hyperplane, (green) extracted from MD simulations using quasiststic hyperplane, and (red) extracted from MD simulations using MD hyperplane.

$\delta\epsilon = 10^{-5}$, and $\epsilon_{end} = 0.1$ for collecting statistics. We sample snapshots with distance between adjacent frames $\sqrt{\sum_i^N \delta\mathbf{r}_i^2} = 0.10$. We then trained hyperplanes using the same protocol, except that structure function placements are:

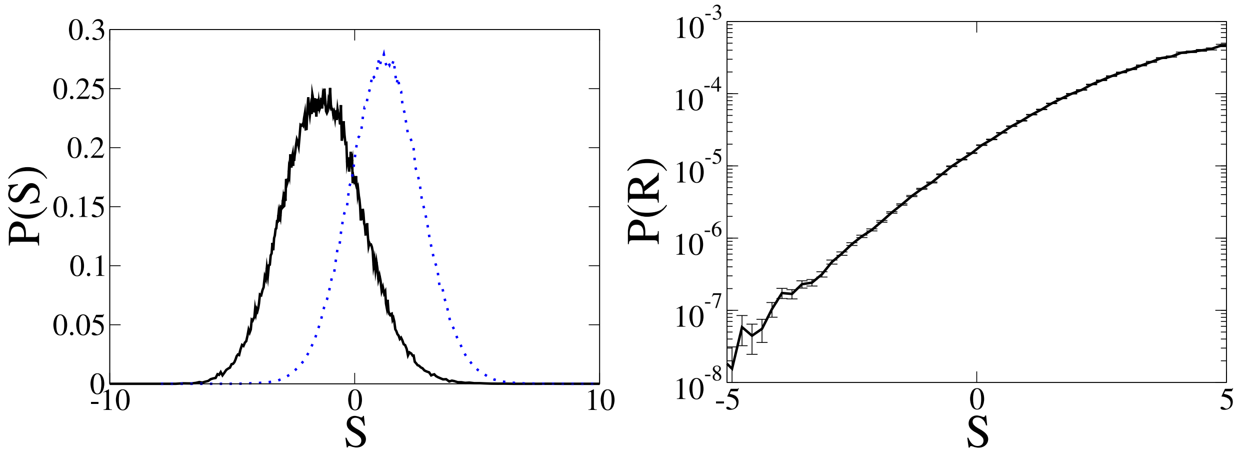


FIG. S5. (a) The distribution of softness for all particles (black solid) and for rearrangers only (blue dotted) in 3D. There is a pronounced difference between the two distributions. (b) The probability that a particle is rearranging, $P_R$, as a function of its softness in 3D. As the softness increases, $P_R$ increases by four orders of magnitude, verifying the high correlation between softness and rearrangements.

| $r_{\text{m, small}}$ | $r_{\text{m, large}}$ |
|---|---|
| $0.8, 0.8 \times 1.04, 0.8 \times 1.04^2, \cdots, 4.86$ | $1, 1.04, 1.04^2, \cdots, 4.99$ |
| $0.8, 0.8 \times 1.04, 0.8 \times 1.04^2, \cdots, 2.92$ | $1, 1.04, 1.04^2, \cdots, 3.00$ |
| $0.8, 0.9, 1.0, \cdots, 5.0$ | $1.0, 1.1, 1.2, \cdots, 5.0$ |
| $0.8, 0.9, 1.0, \cdots, 2.9$ | $1.0, 1.1, 1.2, \cdots, 2.9$ |

and the parameters for training sets are:

| $d_{\text{soft, small}}$ | $d_{\text{soft, large}}$ | $d_{\text{hard, small}}$ | $d_{\text{hard, large}}$ | $\delta\epsilon$ |
|---|---|---|---|---|
| 0.00282 | 0.00086 | 0.03 | 0.02 | 0.1 |
| 0.00141 | 0.00043 | 0.06 | 0.04 | 0.1 |

With hyperplanes trained, we verify the main results of the paper. We show in Fig. S5 that softness is strongly correlated with rearrangements. We then show in Fig. S6 that the deviatoric strain decays roughly as $r^{-3}$, as expected from elasticity theory, and that the softness change follows the volumetric strain. These results provide strong confirmation that our interpretation of the roles of volumetric and deviatoric strain in affecting softness and rearrangements is correct.

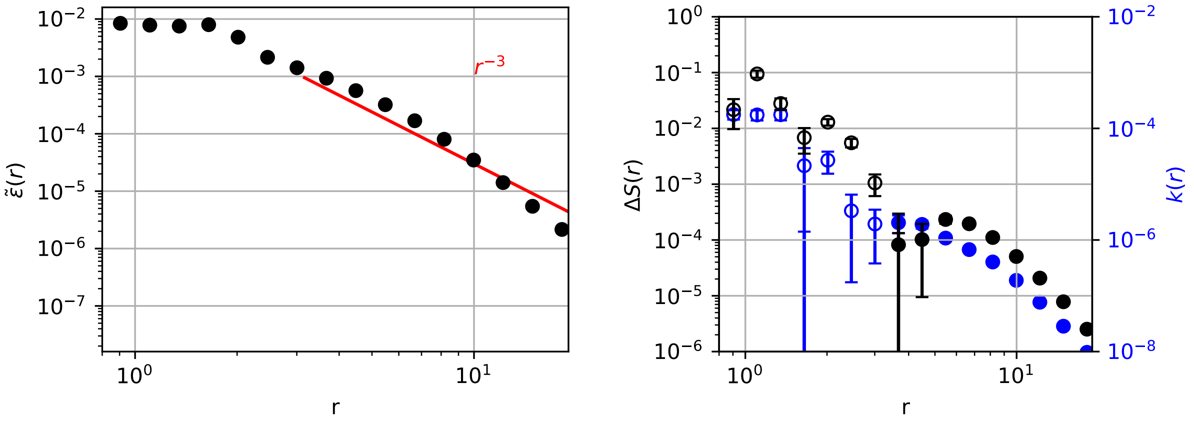


FIG. S6. (left) Mean deviatoric strain $\tilde{\epsilon}$ per frame caused by a rearranger in 3D. Red line indicates $r^{-3}$ scaling predicted by continuum-elasticity theory. (right) Same as left, except for softness change $\Delta S$ and volumetric strain $k$. Same as main-text Figs. 2 and 5, solid circles represent positive values, while open circles represent negative values.

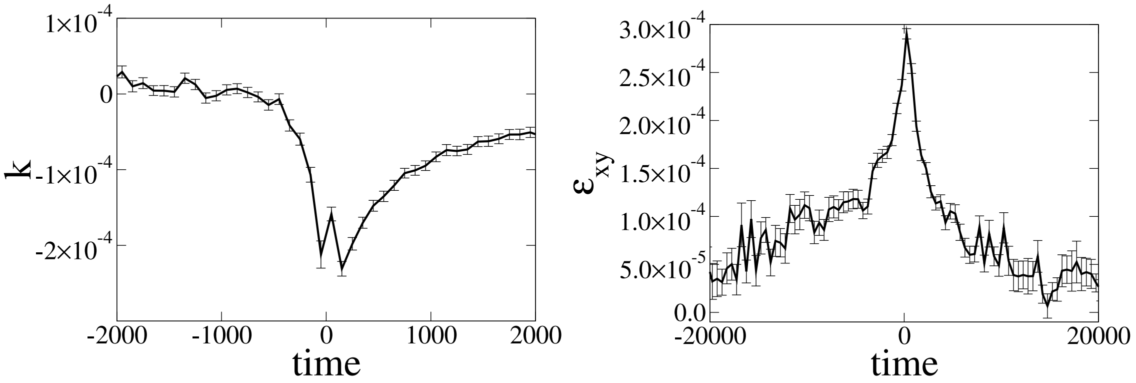


FIG. S7. (left) The local-fit volumetric strain of a rearranger versus time. To average over different rearranging events, they are temporally aligned so that they start ($D^2_{\text{min}}$ raises above the threshold) at $t = 0$. Rearrangements usually end at some time $t$ between $10^2$ and $10^3$. (right) Same as left, except for local-fit $xy$-shear strain.

## VI. LOCAL-FIT STRAINS OF A REARRANGER VERSUS TIME

In Fig. S7, we present the local-fit volumetric and $xy$-shear strains of a rearranger versus time in 2D. The shear strain source persists for a far longer time than the compression source.

[S1] In simulations, $\delta U$ should be calculated using double precision and the Kahan summation algorithm to minimize error.

[S2] S. S. Schoenholz, E. D. Cubuk, D. M. Sussman, E. Kaxiras, and A. J. Liu, Nat. Phys. **12**, 469 (2016).

[S3] T. A. Sharp, S. L. Thomas, E. D. Cubuk, S. S. Schoenholz, D. J. Srolovitz, and A. J. Liu, Proc. Natl. Acad. Sci. **115**, 10943 (2018).
